# Supplementary material for: Tracking Microhydration of the NaCl Rocksalt Molecule in Helium Nanodroplets by Penning Ionization Electron Spectroscopy
Source: arXiv:2510.22000 source file (2025-10-24)
Supplement: Supplementary file 1 [file SM.pdf]

# Supplemental Material: Tracking microhydration of the NaCl rocksalt molecule in helium nanodroplets by Penning ionization electron spectroscopy

L. Ben Ltaief *et al.*

## 1 NaCl doping dependency

Fig. S1 shows PIES of NaCl-doped HNDs recorded at $h\nu = 21.6$ eV for a He nozzle temperature of $T_{\mathrm{nozzle}} = 15$ K ($R = 5$ nm) in panel a) and $T_{\mathrm{nozzle}} = 13$ K ($R = 6$ nm) in b) for various NaCl sample temperatures in the range $T_{\mathrm{NaCl}} = 420$–515°C. The three peaks A, B, and C discussed in the main text are present in all these spectra with variable peak heights for changing $T_{\mathrm{NaCl}}$. The peak integrals of the three features A, B and C as a function of $T_{\mathrm{NaCl}}$ are shown in Fig. S2. Most notably, peaks B and C are more pronounced at the nozzle temperature of 13 K as the HNDs pick up more Na atoms and their photoabsorption cross section is larger, respectively. When $T_{\mathrm{NaCl}}$ is increased, peak B rises sharply presumably due to the thermal desorption of Na from the walls of the vacuum chamber leading to higher doping Na levels; peak C slowly drops because the HNDs shrink as they scatter with NaCl molecules while passing through the NaCl cell.

Peak A, resulting from Penning ionization of NaCl, appears at $T_{\mathrm{NaCl}} \leq 420$°C and increases until it reaches a maximum at $T_{\mathrm{NaCl}} \approx 480$ °C, followed by a drop at higher sample temperatures $T_{\mathrm{NaCl}} > 480$°C. Peak B, due to Penning ionization of Na, increases with $T_{\mathrm{NaCl}}$ reflecting the increasing number of Na atoms picked up by the HNDs as more Na atoms desorb off the chamber walls. Peak C, due to Penning ionization of He$^*$, is independent of any doping of the HNDs. It slightly drops in intensity as a result of shrinking of the HNDs by scattering with NaCl molecules inside the NaCl doping cell.

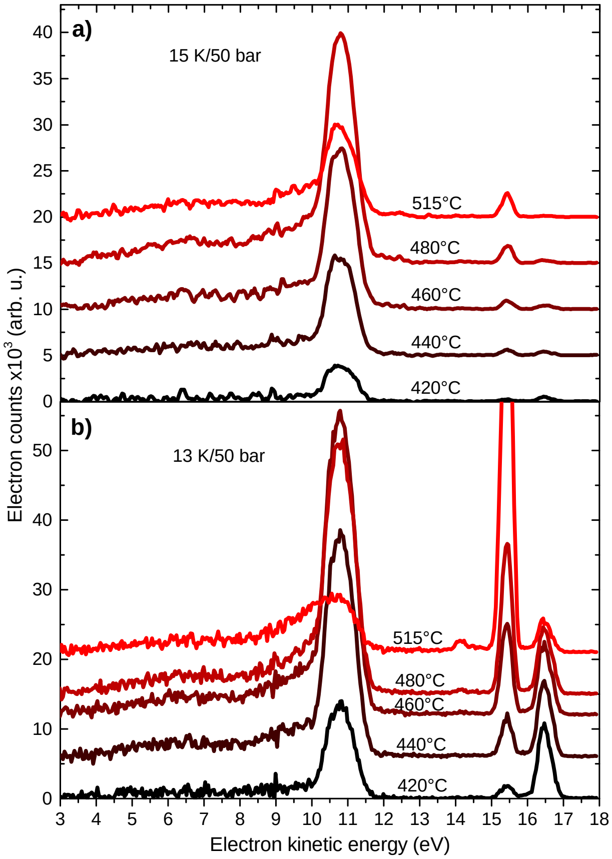


Figure S1: NaCl oven temperature-dependent PIES recorded for NaCl-doped HNDs at $h\nu = 21.6$ eV and at He nozzle temperatures of a) 15 K; and b) 13 K.

At high NaCl oven temperature $T_{\mathrm{NaCl}} > 480°\mathrm{C}$, peak A drops in intensity again due to shrinking of the HNDs and possibly due to inelastic scattering of electrons within the NaCl clusters forming inside the HNDs.

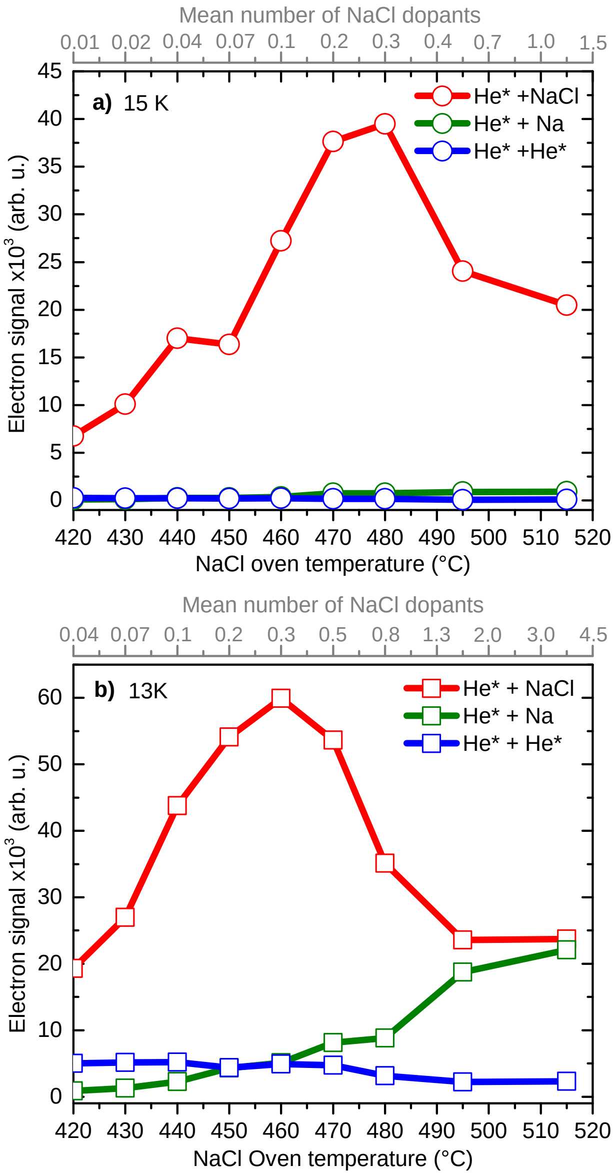


Figure S2: Integrals of the peaks A, B, C in Fig. S1 as a function of temperature of the NaCl doping cell. The mean number of NaCl molecules picked up by the HNDs is shown at the top of panels a) and b), and are estimated using the formulas described in SM section 2.

## 2 Estimation of the mean number of $H_2O$ co-dopant and NaCl dopant molecules

To estimate the mean number $\bar{n}_{\mathrm{H_2O}}$ of $H_2O$ co-dopant molecules picked up by the HNDs, we applied the simple model proposed by Kuma *et al.*,[1]

$$\bar{n}_{\mathrm{H_2O}}(P) = \frac{N_{\mathrm{He}}}{N_{\mathrm{evap}}}\left[1 - \left(1 - \frac{\chi P N_{\mathrm{evap}}}{3N_{\mathrm{He}}}\right)^3\right], \tag{1}$$

where $P$ is the partial pressure of $H_2O$ within the doping region, $N_{\mathrm{He}}$ is the mean number of He atoms per HND,[2] $N_{\mathrm{evap}} = E_{\mathrm{total}}/E_{\mathrm{b(He)}} \approx 1600$ is the number of evaporated He atoms per $H_2O$ molecule picked up by the HND, where $E_{\mathrm{b}}(\mathrm{He}) \approx 5\ \mathrm{cm}^{-1}$ is the average binding energy of a He atom to a HND, and $E_{\mathrm{total}}$ is the total energy released upon the pick up of $H_2O$ dopants. The parameter $\chi$ is given by[1]

$$\chi = \frac{\pi R_{\mathrm{He}}^2 L_{\mathrm{c}}}{k_B T}\sqrt{\frac{v_d^2 + v_m^2}{v_d^2}}, \tag{2}$$

where $L_{\mathrm{c}}$ is the length of the doping cell and $R_{\mathrm{He}}$ is the effective radius of the HND defined as $R_{\mathrm{He}} = (\frac{3N_{\mathrm{He}}}{4\pi r_0})^{1/3}$. Here, $r_0 \approx 2.18 \times 10^{28}\ \mathrm{m}^{-3}$ is the density of superfluid He, $v_d$ is the mean velocity of the HND beam,[3] and $v_m$ is the mean thermal velocity of $H_2O$ molecules that can be calculated using the kinetic theory of gases, $v_m = \sqrt{\frac{8k_{\mathrm{B}}T}{\pi m_{\mathrm{H_2O}}}}$ where $k_{\mathrm{B}}$ is the Boltzmann constant, $T$ is the temperature of the doping cell, and $m_{\mathrm{H_2O}}$ is the molecular mass of $H_2O$.

The pressure $P$ in Eq. (1) is defined as

$$P = \frac{4S(p - p_{\mathrm{bkg}})}{A v_m} + \frac{(p - p_{\mathrm{bkg}})L_{\mathrm{ch}}}{L_c}, \tag{3}$$

where $p$ and $p_{\mathrm{bkg}}$ is the pressure of the chamber after and before co-doping with $H_2O$ molecules, respectively. $S$ is the effective pumping speed of the pump attached to the doping chamber, $L_{\mathrm{ch}}$ is the length of the doping chamber, and $A = \frac{\pi}{4}\left(d_1^2 + d_2^2\right)$ is the total open area of the holes in the doping cell with diameters $d_1$ and $d_2$.

Note that $E_{\mathrm{total}}$ used in Eq. (1) to estimate $N_{\mathrm{evap}}$ is calculated according to the formula described in Ref. 4, which is the sum of the internal

rovibrational energy of the $H_2O$ dopant $E_{\mathrm{int}} = (N/2)k_{\mathrm{B}}T$, $N = 6$ being the number of degrees of freedom (rotation and vibration) of the water molecule, and the collision energy between the $H_2O$ dopants and the HND, $E_{\mathrm{coll}} = \left(\frac{3}{2}k_{\mathrm{B}}T + \frac{1}{2}m_{\mathrm{H_2O}}v_{\mathrm{d}}^2\right)$, the relative binding energy of one $H_2O$ molecule interacting with one He atom $E_b(\mathrm{He–H_2O})$ [5,6] and with another $H_2O$ molecule $E_b(\mathrm{H_2O–H_2O})$ [4,7] and the average relative binding energy of 8 $H_2O$ molecules surrounding one dopant NaCl molecule $\frac{1}{8}\sum_{n=1}^{8} E_{\mathrm{b}}(\mathrm{H_2O}_n\mathrm{-NaCl})$ [See figure 8 in the main text].

Table 1: Parameters used to estimate $\bar{n}_{\mathrm{H_2O}}$ and $\bar{n}_{\mathrm{NaCl}}$ for optimum droplet and doping conditions ($T_{\mathrm{nozzle}}$/He backing pressure = 13 K/50 bar, $T_{\mathrm{NaCl}}$ = 460°C).

| **Symbol** | **NaCl** | **$H_2O$** | **Units** | **References** |
|---|---|---|---|---|
| $S$ | 0.685 | 0.685 | $m^3/s$ | |
| $d_1$ | 0.002 | 0.0035 | m | |
| $d_2$ | 0.003 | 0.004 | m | |
| $L_c$ | 0.01 | 0.018 | m | |
| $L_{ch}$ | 0.32 | 0.32 | m | |
| $m$ | 58 | 18 | amu | |
| $v_m$ | 627 | 594 | m/s | |
| $v_d$ | 320 | 320 | m/s | [Ref. 3] |
| $N_{\mathrm{He}}$ | $\sim 10^5$ | $\sim 10^5$ | | [Ref. 2] |
| $T$ | 733.15 | 300 | K | |
| $E_{\mathrm{int}}$ | 94.8 | 77.5 | meV | |
| $E_{\mathrm{coll}}(\mathrm{HND-NaCl})$ | 125.6 | | meV | |
| $E_{\mathrm{coll}}(\mathrm{HND-H_2O})$ | | 48.32 | meV | |
| $E_b(\mathrm{He-NaCl})$ | 2.2 | | meV | [This work] |
| $E_b(\mathrm{He-H_2O})$ | | 32 | meV | [Refs. 5,6] |
| $E_b(\mathrm{NaCl-NaCl})$ | 2000 | | meV | [Ref. 8] |
| $E_b(\mathrm{H_2O-H_2O})$ | | 233.61 | meV | [Refs. 4,7] |
| $\frac{1}{8}\sum_{n=1}^{8} E_{\mathrm{b}}(\mathrm{H_2O}_n\mathrm{-NaCl})$ | | 600 | meV | [This work] |

Unlike the case of doping with $H_2O$ gas molecules, where the partial pressure $P$ is inferred from pressure measured at the doping chamber, doping NaCl molecules into HNDs requires heating of the NaCl sample to generate vapor. The NaCl partial pressure $P$ is calculated from the temperature $T$ of

the heated doping cell using the simplified empirical relation[9]

$$\log_{10} P = A - \frac{B}{T}, \tag{4}$$

where $A = 10.41$ and $B = 11600.51$ are constants specific to the sublimation properties of NaCl. By substituting this value of $P$ in Eq. (1), the average number of NaCl molecules $\bar{n}_{\mathrm{NaCl}}$ picked up by the HNDs can be reliably estimated as a function of $T$. The mean number of evaporated He atoms ($N_{\mathrm{evap}}$) per one doped NaCl diatomic molecule (with $N = 3$ degrees of freedom) as well as the $\chi$ parameter are calculated in the same way as described above for the case of $H_2O$ doping. $N_{\mathrm{evap}}$ reads about 3738, for example, at $T$nozzle/He backing pressure = 13 K/50 bar ($N_{\mathrm{He}} \sim 10^5$) and $T_{\mathrm{NaCl}}$= 460°C. Table 1 summarizes the key parameters used in this work to estimate $\bar{n}_{\mathrm{H_2O}}$ and $\bar{n}_{\mathrm{NaCl}}$ under the optimum droplet and doping conditions ($T$nozzle = 13 K, He backing pressure = 50 bar, $T_{\mathrm{NaCl}}$ = 460°C). These parameters are also applicable to any other droplet and doping conditions.

# 3 Details of the replica-exchange molecular dynamics simulations

For each cluster size, and any umbrella potential imposing an approximate $Na^+$–$Cl^-$ distance, a ladder of 40 temperatures, geometrically distributed in the range 10–200 K, was employed, with individual MD trajectories consisting of $10^8$ time steps, following $2 \times 10^7$ equilibration steps, and a time step of 0.5 fs. Occasional exchanges between random pairs of adjacent replicas were attempted every picosecond. By varying the Na-Cl distance between 1.5 and 6 Å by steps of 0.5 Å, large samples of configurations gathered in the 10 lowest temperature REMD trajectories could finally be subjected to local minimization, eventually producing sets of candidate structures to be refined at the quantum chemistry level.

# 4 Equilibrium configuration of NaCl embedded in HNDs

Penning ionization is sensitive to the local environment of the compounds being probed. Therefore, we investigated the equilibrium configuration of NaCl

relative to the droplet center in the absence of water co-dopants. For this purpose, two complementary types of simulations were conducted; one using the continuum-based He-density-functional theory ($^4$He-DFT) approach,[10] and the other one based on path-integral molecular dynamics (PIMD) method, directly at the atomistic level of details.[11]

## 4.1 He-DFT approach

$^4$He-DFT has proven to be the best compromise between accuracy and the ability to treat a large number of He atoms, as explained in Ref. 10 where details about the method can be found. The $^4$He-DFT simulations were performed using the free and open-source 4He-DFT-BCN-TLS code[12] with the Orsay-Trento functional[13] to which we add an additional term that only acts when the density is very high, close to that of the solid phase.[14,15] The NaCl molecule was represented by treating the ions as classical particles and the rest of the droplet by its continuous He density, both expanded on the same 3-dimensional Cartesian grid. The equilibrium configuration was found by solving the coupled Euler-Lagrange equations arising from the functional variation of the equation expressing the total energy as a functional of the He density.

The NaCl-droplet interaction was taken as a sum of pairwise NaCl-He potentials obtained from cuts through the three-dimensional potential energy surface. Reference data for the potential energy surface for a NaCl molecule interacting with a He atom were computed at the CCSD(T)/AVQZ level of theory (without core) and performing the basis set superposition error correction in a way similar to earlier calculations on the OCS molecule embedded in HNDs.[14,15]

Cuts of the potential along different orientations with respect to the NaCl molecular orientations are shown in Fig. S3. The strongest bond occurs for the linear He-NaCl configuration where the He atom locates itself at a distance of 3.7 Å from the $Na^+$ ion. For this configuration, the well depth amounts to $E_b = 150$ K$\times k_{\mathrm{B}}$, corresponding to 13 meV. In the linear NaCl-He configuration and in the T-shaped configurations, the binding potential is much shallower, $E_b = 30$ K$\times k_{\mathrm{B}}$ (2.6 meV) and $E_b = 25$ K$\times k_{\mathrm{B}}$ (2.2 meV). Here, $k_{\mathrm{B}}$ is the Boltzmann constant.

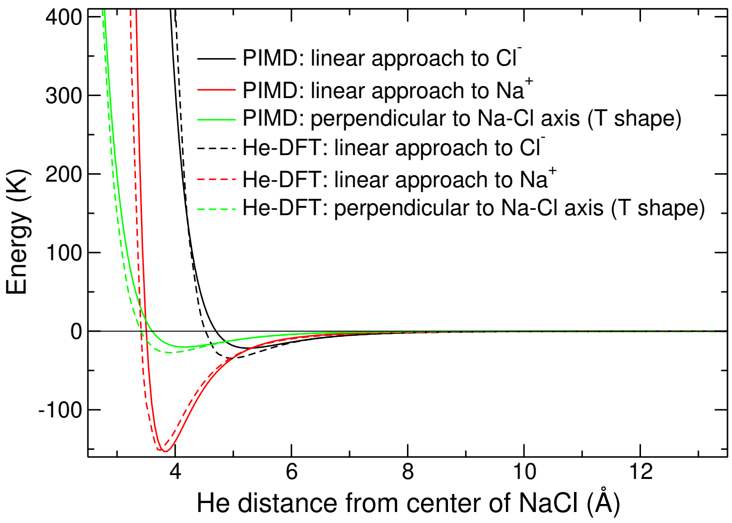


Figure S3: Symbols: Potential energy curves for a ground state NaCl molecule interacting with a He atom at various orientations with respect to the NaCl molecular axis, used in the $^4$He-DFT simulations (dashed lines) or in the PIMD simulations (solid lines).

## 4.2 PIMD simulations

Alternatively to the $^4$He-DFT approach, PIMD simulations at equilibrium were also performed for NaCl embedded in small helium nanodroplets. At variance with the $^4$He-DFT method, bosonic exchange is neglected in the presently used conventional PIMD approach, hence any effects arising from superfluidity are practically neglected. Yet, the method can tackle large systems, too, and, in the present case, did not rely on the $Na^+$ and $Cl^-$ ions being fixed in the reference frame. In earlier work,[16] the relative performances of the $^4$He-DFT and path-integral-based atomistic approaches were compared for specific time-dependent problems. Here, PIMD simulations were performed at 2 K thermal equilibrium, using a Trotter discretization number of $P = 64$ following the methodology described in the above reference.[16]

In the PIMD model of the NaCl embedded in $He_n$ droplets, the $Na^+$, $Cl^-$ ions and all He atoms are treated as individual particles interacting through

dedicated potentials. More precisely, we use an additive potential as

$$\begin{aligned} V(\mathbf{R}) &= \sum_{i\in \mathrm{He}} V_{\mathrm{Na^+He}}(r_i) + \sum_{i\in \mathrm{He}} V_{\mathrm{Cl^-He}}(r_i) \\ &+ V_{\mathrm{NaCl}}(r_{\mathrm{NaCl}}) + \sum_{i,j\in \mathrm{He}} V_{\mathrm{HeHe}}(r_{ij}) \\ &+ \sum_{i\in \mathrm{He}} V_{\mathrm{pol}}^{(i)} \end{aligned} \tag{5}$$

where we have generally denoted by $\mathbf{R}$ the entire set of Cartesian coordinates, $r_i$ the distance between He atom $i$ and either $Na^+$ or $Cl^-$ ion, $r_{ij}$ the distance between the two He atoms $i$ and $j$.

The interaction between the two ions is modeled using a very conventional Born-Mayer+Coulomb form,

$$V_{\mathrm{NaCl}}(r) = A\exp(-br) - 1/r. \tag{6}$$

The interactions between He atoms and the two ions comprise of a long-range polarization contribution that is included in the term $V_{\mathrm{pol}}$, plus some shorter-range term notably accounting for Pauli repulsion. Morse expressions were found to be more accurate than power-law forms to reproduce quantum chemical data:

$$V_{\mathrm{X^\pm He}}(r) = V_0\{\exp[-2\rho(r-r_0)] - 2\exp[-\rho(r-r_0)]\}, \tag{7}$$

where $X^\pm$ denotes either $Na^+$ or $Cl^-$. The polarization term $V_{\mathrm{pol}}^{(i)}$ affecting He atom $i$ is taken at the level of approximation just beyond the pair order of $-1/r^4$, through the expression

$$V_{\mathrm{pol}}^{(i)} = -\frac{\alpha_{\mathrm{He}}}{2}\vec{E}_i^2, \tag{8}$$

where $\vec{E}_i$ is the electric field on the He atom created by the sodium and chloride ions. Finally, and for computational efficiency, the He-He interaction was chosen to be a simple Lennard-Jones pairwise potential with parameters chosen to reproduce the more accurate Jenzen-Aziz potential[17], namely $\varepsilon = 3.404 \times 10^{-5}$ Hartree and $\sigma = 4.982\ a_0$, where $a_0$ is the Bohr radius.

Other than the He-He interactions, the various parameters of this potential were determined by fitting the appropriate functional forms to quantum chemical data performed at the CCSD(T)/aug-cc-pV5Z level of theory, leading to the following values of $A = 4.603$ Hartree, $b = 4.343 \times$

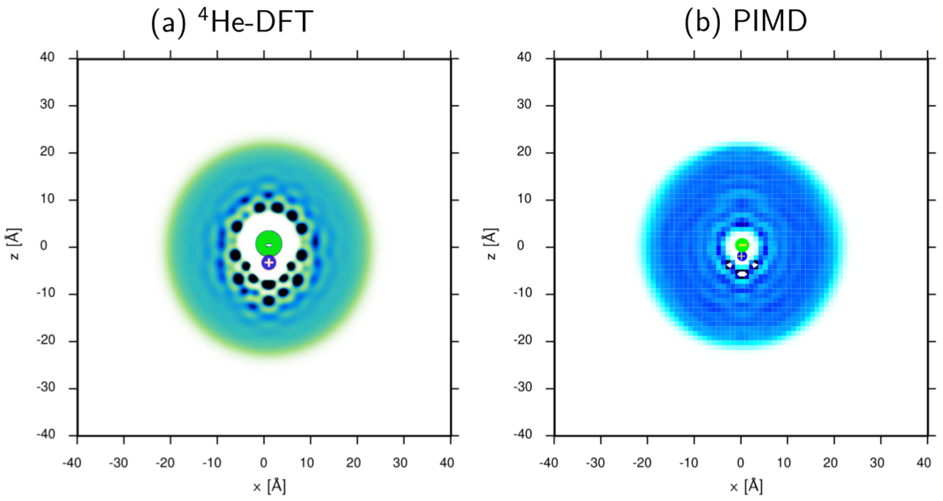


Figure S4: Helium density profile for a 1000-atom droplet around the NaCl molecule located at the center. (a) $^4$He-DFT continuum calculation; (b) Atomistic PIMD simulations. In both plots, the $Na^+$ and $Cl^-$ ions are represented by blue (⊕) and green (⊖) balls, respectively. The color scales are mainly indicative of the physical extension of the droplets.

$10^{-4}\ a_0^{-1}$, $V_0(\mathrm{Na}^+) = 1.048\times10^{-4}$ Hartree, $r_{\mathrm{Na}^+} = 5.349\ a_0$, $\rho_{\mathrm{Na}^+} = 1.218\ a_0^{-1}$, $V_0(\mathrm{Cl}^-) = 2.452 \times 10^{-5}$ Hartree, $r_{\mathrm{Cl}^-} = 8.820\ a_0$, and $\rho_{\mathrm{Cl}^-} = 0.692\ a_0^{-1}$. The experimental value was employed for the atomic polarizability of He, $\alpha = 1.383\ a_0^3$.

The resulting interaction potentials between He and the NaCl molecule at equilibrium are superimposed in Fig. S3. The agreement with the potential used in the $^4$He-DFT calculations is satisfactory, given the different underlying approximations in the treatment of the ionic molecule. In particular, the preferred equilibrium position near the sodium cation is correctly reproduced both in terms of distance and well depth.

## 4.3 Density distributions at equilibrium

The equilibrium densities of HNDs containing 1000 atoms, as obtained using the $^4$He-DFT and PIMD methods, are represented in Fig. S4(a) and S4(b), respectively.

Comparison of these plots shows various interesting features that are robust against the computational method, starting with the natural preference

of the NaCl molecule to be fully submerged in the HND where it resides at the center. It is also remarkable that the asymmetry in the interaction between He and the two $Na^+$ and $Cl^-$ ions is reflected on both density plots, the $Na^+$ cation binding far more strongly to the He solvent than the $Cl^-$ anion, resulting in a more localized 'snowball' shell on the $Na^+$ side of the molecule.

# References


[1] S. Kuma, H. Goto, M. N. Slipchenko, A. F. Vilesov, A. Khramov and T. Momose, *J. Chem. Phys.*, 2007, **127**, 214301.

[2] J. P. Toennies and A. F. Vilesov, *Angew. Chem., Int. Ed. Engl.*, 2004, **43**, 2622–2648.

[3] L. F. Gomez, E. Loginov, R. Sliter and A. F. Vilesov, *J. Chem. Phys.*, 2011, **135**, 154201.

[4] S. De, A. Abid, J. Asmussen, L. Ben Ltaief, K. Sishodia, A. Ulmer, H. Pedersen, S. Krishnan and M. Mudrich, *J. Chem. Phys.*, 2024, **160**, 094308.

[5] M. Lewerenz, B. Schilling and J. Toennies, *J. Chem. Phys.*, 1995, **102**, 8191–8207.

[6] S. Green, D. DeFrees and A. McLean, *J. Chem. Phys.*, 1991, **94**, 1346–1359.

[7] A. Malloum, J. J. Fifen, Z. Dhaouadi, S. G. N. Engo and J. Conradie, *New J. Chem.*, 2019, **43**, 13020–13037.

[8] D. Welch, O. Lazareth, G. Dienes and R. Hatcher, *J. Chem. Phys.*, 1976, **64**, 835–839.

[9] G. W. Thomson, *Chemical reviews*, 1946, **38**, 1–39.

[10] F. Ancilotto, M. Barranco, F. Coppens, J. Eloranta, N. Halberstadt, A. Hernando, D. Mateo and M. Pi, *Int. Rev. Phys. Chem.*, 2017, **36**, 621–707.

[11] A. Pérez, M. E. Tuckerman and M. H. Müser”’, *J. Chem. Phys.*, 2009, **130**, 184105.

[12] *4He-DFT-BCN-TLS/He_DFT_2017*, 4He-DFT BCN-TLS, 2024, https://github.com/4He-DFT-BCN-TLS/He_DFT_2017.

[13] F. Dalfovo, A. Lastri, L. Pricaupenko, S. Stringari and J. Treiner, *Phys. Rev. B*, 1995, **52**, 1193–1209.

[14] F. Ancilotto, M. Barranco, F. Caupin, R. Mayol and M. Pi, *Phys. Rev. B*, 2005, **72**, 214522.

[15] D. Mateo, F. Gonzalez and J. Eloranta, *J. Phys. Chem. A*, 2015, **119**, 2262–2270.

[16] E. García-Alfonso, M. Barranco, D. A. Bonhommeau, N. Halberstadt, M. Pi and F. Calvo, *J. Chem. Phys.*, 2022, **157**, 014106.

[17] A. R. Janzen and R. A. Aziz, *J. Chem. Phys.*, 1997, **107**, 914–919.
